# Supplementary material for: Interpreting Deep Learning Model Using Rule-based Method
Source: arXiv:2010.07824 source file (2020-10-15)
Supplement: Supplementary file 1 [file appendix.tex]

\newpage

??

\newpage

\appendix

\section{Supplemental Materials}

%We offer some reproducibility-related information as supplemental materials.
\subsection{Datasets}

In the experiments, we test our model with over three popular image datasets, which are Fashion-MNIST, CIFAR-10 and ImageNet. All pixels in the image data are projected into [0, 1].

$\bullet$ Fashion-MNIST~\cite{xiao2017fashion} is a dataset comprising of 28$\times$28 grayscale images of 70,000 fashion products from 10 categories, with 7,000 images per category. The training set has 60,000 images and the test set has 10,000 images.

$\bullet$ CIFAR-10~\cite{krizhevsky2009cifar} contains 60,000 color images corresponding to 10 different object classes. In the dataset, 10,000 images are for training and 50,000 for testing. The image size is 32$\times$32.

$\bullet$ ImageNet~\cite{imagenet_cvpr09} is a large natural image dataset containing over 1.2 million images. We select images of 20 object classes from the dataset for our experiment. Each class contains 1,040 training samples and 260 test samples. All these images are resized to 256$\times$256 and center cropped to 224$\times$224. The label indexes of the chosen objects are 7, 30, 36, 58, 75, 101, 161, 282, 398, 456, 496, 510, 549, 620, 696, 734, 752, 908, 954, 980 (from 0 to 999).

\subsection{Experiment Environments}

Our software environment contains ubuntu 18.04, PyTorch v1.1.0 and python 3.6.5 (we also use Tensorflow v1.12 for baseline PixelDefend). All of the experiments are conducted on a machine with four GPUs (NVIDIA GeForce GTX 2080 Ti * 4), one CPU (Intel(R) Xeon(R) Silver 4210 CPU @ 2.20GHz) and 128G memory.

\subsection{Model Structures}

% Table generated by Excel2LaTeX from sheet 'Sheet4'
\begin{table}[h] \footnotesize
  \centering
  \caption{Model structures in our experiments for each dataset and component.}
   \resizebox{0.9\columnwidth}{!}{
    \begin{tabular}{c|c|c|c}
    \toprule
      & \makecell{Fashion\\-MNIST} & CIFAR-10 & ImageNet  \\
    \toprule
    \makecell{Target\\ Classifier } & VGG11\cite{vgg11} & VGG11\cite{vgg11} & InceptionV3\cite{incepv3}  \\
    \midrule
    \makecell{Black-box \\Classifier } & CWnet\cite{carlini2017cw} & Wide-ResNet\cite{rony2019ddn} & ResNet152\cite{resnet}  \\
    \midrule
    Detector & VGG11\cite{vgg11} & VGG11\cite{vgg11} & VGG11\cite{vgg11}  \\
    \midrule
    Rectifier & VGG11\cite{vgg11} & VGG11\cite{vgg11} & VGG16\cite{vgg11}  \\
    \midrule
    \makecell{Adversarial \\Training} & VGG11\cite{vgg11} & VGG11\cite{vgg11} &  InceptionV3\cite{incepv3} \\
    \bottomrule
    \end{tabular}%
    }
  \label{tab:model structure}%
\end{table}%

Table \ref{tab:model structure} lists the model structures in our experiments, including the attacker target classifier (also our protected classifier), the detector and rectifier model in our X-Ensemble Model, adversarial training model for baselines. In the black-box evaluation we use the black-box classifier to generate adversarial examples and then perform transferable attacks on the target classifier. Notice that the input image size of InceptionV3 should be 299$\times$299, but we set the image size as 224$\times$224 for InceptionV3, which is also supported by PyTorch, to reduce the computational cost when generating adversarial examples and also to fit the input size of ResNet152. We only use pre-trained InceptionV3 of target classifier and pre-trained ResNet152 of black-box classifier by PyTorch. When using these models, we select the output logits of those 20 chosen classes and then compute the probabilities for them with $softmax$ function. In this way, InceptionV3 and ResNet152 both have 95\% accuracy on the ImageNet subset.

\subsection{Setting of Attackers}

The codes of attack methods are implemented by AdverTorch v0.2. Table \ref{tab:attack para} reports the attacking parameters in this paper.

% Table generated by Excel2LaTeX from sheet 'Sheet4'
\begin{table}[ht] \footnotesize
  \centering
  \caption{Attacking parameters for generating adversarial examples. }
   \resizebox{0.9\columnwidth}{!}{
    \begin{tabular}{c|c|c|c|c}
    \toprule
    Attacker & Parameter & \makecell{Fashion\\-MNIST} & CIFAR-10 & ImageNet \\
    \midrule
    FGSM & $\epsilon$ & 0.031 & 0.031 & 0.031 \\
    \midrule
    \multirow{3}[6]{*}{PGD} & $\epsilon$ & 0.031 & 0.031 & 0.031 \\
\cmidrule{2-5}      & iteration & 20 & 20 & 20 \\
\cmidrule{2-5}      & $\alpha$ & 0.00781 & 0.00781 & 0.00781 \\
    \midrule
    {Dfool}     & iteration & 100 & 100 & 30 \\
    \midrule
    \multirow{3}[6]{*}{CW} & learning rate & 0.01 & 0.01 & 0.01 \\
\cmidrule{2-5}      & iteration & 100 & 100 & 50 \\
\cmidrule{2-5}      & $c$ & 0.01 & 0.01 & 0.01 \\
    \midrule
    DDN & iteration & 100 & 100 & 50 \\
    \bottomrule
    \end{tabular}%
    }
  \label{tab:attack para}%
\end{table}%

The $\epsilon$ in FGSM and PGD is to constrain the $L_{\infty}$ perturbation of adversarial examples. The $\alpha$ in PGD and the learning rate in CW control the step size in each iteration when searching perturbation. The higer $c$ in CW is to construct adversarial example with more confidence to fool the classifier. Iteration limits how many times that an iterative attack can compute. Other parameters use their default values in AdverTorch. Targeted and untargeted attacks share the same parameters.These parameters also work for generating adversarial examples in the black-box evaluation.

\paratitle{Adversarial Specificities.} These attacks have two types of adversarial specificities, \ie untargeted attacks and targeted attacks~\cite{akhtar2018threat}:

$\bullet$ {\em Untargeted Attack.} For an image with an original predicted label of $\hat{y}^\circ$, its untargeted adversarial counterpart is successful when the perturbed predicted label $\hat{y}'$ satisfies $\hat{y}' \neq \hat{y}^\circ$.

$\bullet$ {\em Targeted Attack.} For an image with an original predicted label $\hat{y}^\circ$, its targeted adversarial counterpart is successful only when the perturbed label $\hat{y}'$ satisfies $\hat{y}' = y^{(t)}$ and $y^{(t)} \neq \hat{y}^\circ$. In our experiments, the given targeted label $y^{(t)}$ is chosen randomly.

%We implement ADV2 attack on our own and the optimizer is based on PGD. For experiments on Fashion-MNIST, the perturbation constrain $\epsilon$ is set as 0.031, and the iteration is set to 60 with first 30 steps for warm start with PGD attack. For experiments on CIFAR-10, $\epsilon$ is set as 0.031, and the is set to 40, with first 20 epochs for warm start.

\subsection{Interpretation Methods}

We implement VG, GBP and IG methods on our own and use LRP code from~\cite{montavon2019layer}. The integrated step in IG is set to 50. Note that LRP from~\cite{montavon2019layer} cannot be applied on InceptionV3 and ResNet152 directly. So we remove LRP detector only for ImageNet.

\subsection{Baselines}

\begin{itemize}
\item \textbf{PD} The code is from BPDA\footnote{https://github.com/anishathalye/obfuscated-gradients/tree/master/pixeldefend}. When purifying images, $\epsilon$ is set to 0.125 for Fashion-MNIST and 0.063 for both CIFAR-10 and ImageNet. The pretrained model of PixelCNN for CIFAR-10 is from $openai^2$, and we train PixelCNN on Fashion-MNIST and ImageNet with code from $openai$ \footnote{https://github.com/openai/pixel-cnn}.
\item \textbf{TWS} The code is from \cite{hu2019new}. We set the parameters n\_radius = 0.01, targeted\_lr = 0.0005, t\_radius = 0.5, u\_radius = 0.5 and untargeted\_lr = 1.
\item \textbf{MHL} The code is from \cite{lee2018simple}. The magnitude of noise starts from 0.05 to 0.3 with an interval of 0.05 to compute its AUC.
\item \textbf{TVM} The code is from~\cite{tvm}. We set TVM\_WEIGHT = 0.03, PIXEL\_DROP\_RATE = 0.5, TVM\_METHOD = 'tvl2'.
\end{itemize}

\subsection{Training Details}

\begin{itemize}
\item \textbf{Classifier} We use Fashion-MNIST and CIFAR-10 to train their target classifiers and black-box classifiers. The initial learning rates are 0.1 and 0.01 and the training epochs are 20 and 30 respectively. The classifiers for ImageNet are pretrained by PyTorch.
\item \textbf{Detector} We first use the attack methods to generate adversarial examples on the dataset. And then the benign images and corresponding perturbed images are fed to train the data detector. Next, we use the interpreting method to generate their interpreting maps and train interpreting detectors(VG, GBP, IG, LRP).  The label of benign, $L_{\infty}$ perturbed and $L_2$ perturbed examples are 0, 1 and 2. The initial learning rate are set to 0.01 and detectors are trained with 30 epochs.
\item \textbf{Rectifier} We use Alg. \ref{algo:masked_image} to compute masked images on adversarial examples and the sensitivity of $\alpha$ is reported in Fig. \ref{fig:alpha}. As we can see, the original classifier have high accuracy on those $L_2$ masked images. Here the figure of Fashion-MNIST is omitted since its sensitivity is similar to ImageNet. We set $\alpha$ to 0.6, 0.9, 0.5 for Fashion-MNIST, CIFAR-10 and ImageNet. And we find that rectifier trained with masked images of DDN-T mixed with clean images have better performance.
\end{itemize}

\begin{figure}[t]
\begin{center}
    \subfigure[CIFAR-10]{\includegraphics[width=0.49\columnwidth]{./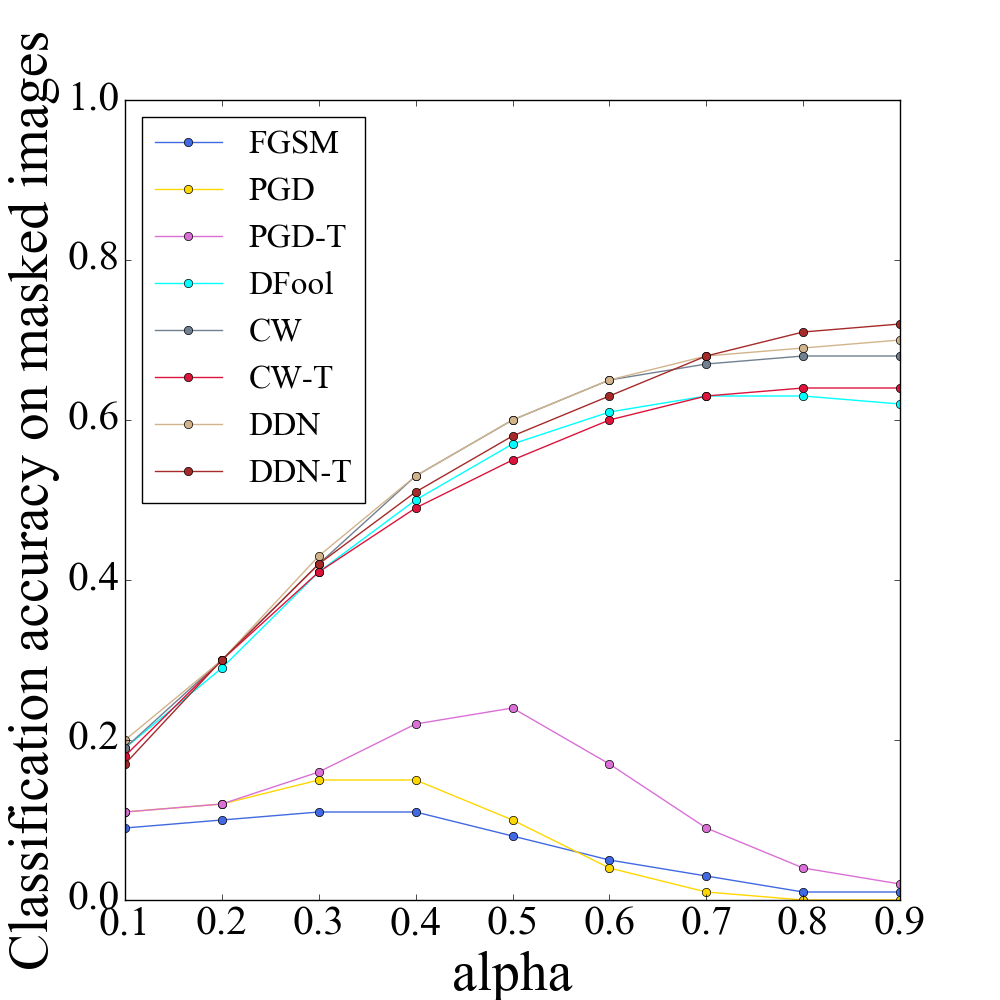}}
   \subfigure[ImageNet]{\includegraphics[width=0.49\columnwidth]{./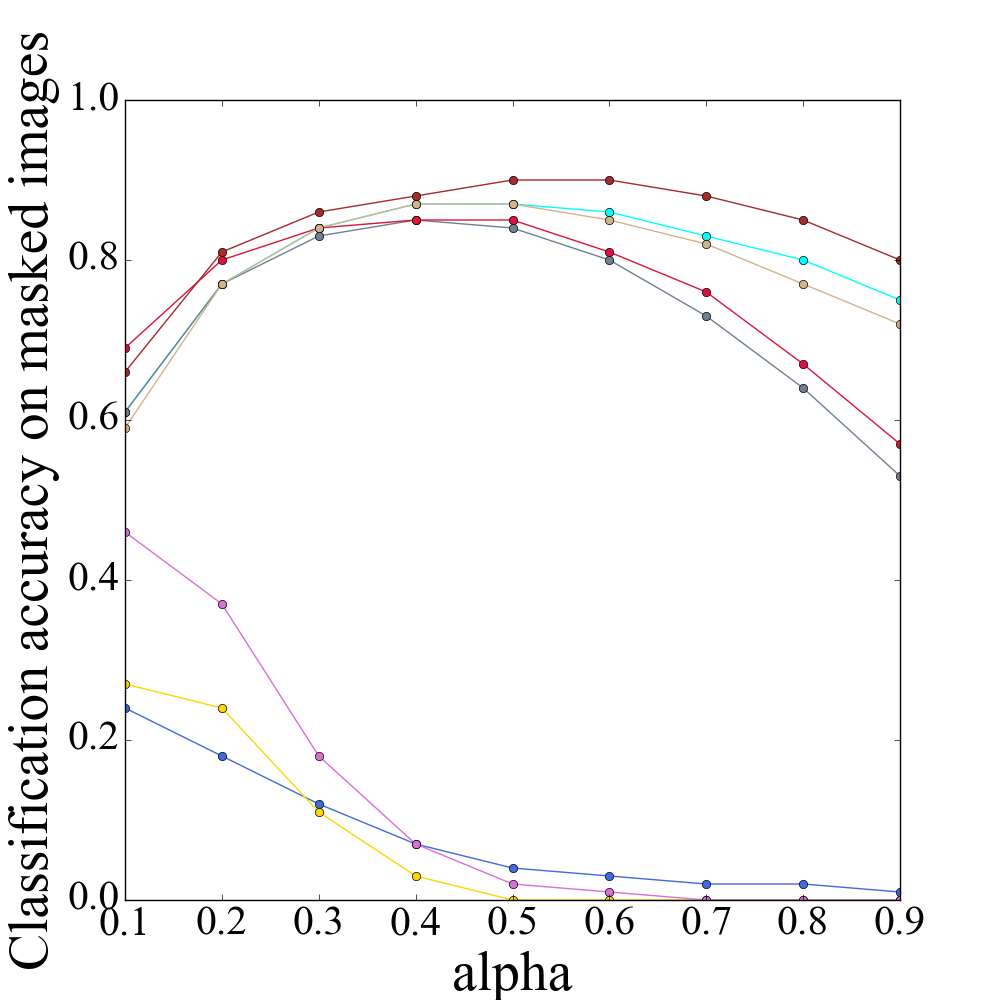}}
\end{center}
\caption{$\alpha$ parameter sensitivity}
\label{fig:alpha}
\end{figure}

\begin{algorithm} [t]
    %\algloopdefx{with}[1]{\textbf{with} #1 \textbf{then}}
\caption{Masked Image For Training Rectifier}\label{algo:masked_image}
\begin{algorithmic}[0]
    \STATE {\bf Variables:} $\{D_1,...,D_J\}$ are the sub-detectors that predict an image as an adversarial one, $\alpha \in (0,1)$ is a threshold parameter, $rand()$ returns a random value in $[0, 1]$, $\sigma$ is variance of pixel values in $x$.
    %\PROCEDURE{GET MASKED IMAGE}{$x, D_1,...,D_j, \alpha$}
    \FOR{$k=1$ to $j$ }
        \STATE $E_k \gets Entropy(D_k(x))$
    \ENDFOR
    \STATE $D \gets D_i$ where $i=argmin(E_1,...,E_j)$
    \STATE $g \gets \frac{\partial \mathcal{L}(D(x))}{\partial x}$
    \STATE $thres \gets \alpha*(\max(g)-\min(g)) + \min(g)$
    \FOR{ Pixel\ $(i,j)$ in $x$}
        \IF{$g_{i,j} > thres$ \textbf{and} $ rand() > 0.5$}
        \STATE $x_{i,j} \gets x_{i,j} + Normal(0, \sigma)$
        \ENDIF
    \ENDFOR
    \STATE \textbf{return} $x$
    %\ENDPROCEDURE
    %\STATE {\bf end Procedure}
\end{algorithmic}
\end{algorithm}

\subsection{White-box Attacker for \name}

In Ref.~\cite{carlini2017adversarial} proposed to combine a classifier and a neural network detector into a new classifier $G$ with L+1 classes, whose ${(L+1)}^{th}$ label identify an input as adversarial. In this way, an attacker can directly attack $G$ to break $F$ and $D$ at the same time. $G$ is defined as,
\begin{equation}
%\begin{align}
    G(x)_i =
    \left\{ \begin{array}{lcr}
    F(x)_i &~~~ \mathrm{if}~~ i \leq L \\
    (D(x)+1) \cdot max_jF(x)_j &~~~ \mathrm{if}~~  i = L+1
     \end{array} \right.
     \label{equ:n+1classifier}
%\end{align}
\end{equation}
where if $x$ is clean then $D(x) < 0$, so we have $G(x)_{L+1} > max(F(x))$ and  $argmax_i G(x)_i = L+1$; if $x$ is adversarial then $D(x) > 0$, so we have $argmax_i G(x)_i = argmax_i F(x)_i$.

From the definition, when an attacker tries to use targeted attack ( with a target $t \neq l$ and $t \neq L+1$) to construct adversarial examples on $G$, it will optimize the examples with a joint objective.

In our experiment, an attacker needs to fool all the detectors in \name. So we modify $G$ into an L+4 classifier as,
\begin{equation}
%\begin{align}
    G(x)_i =
    \left\{ \begin{array}{lcr}
    F(x)_i &~~~ \mathrm{if}~~ i \leq L \\
    (D_k(x) + 1) \cdot max_jF(x)_j &~~~ \mathrm{if}~~  i = L+k
     \end{array} \right.
     \label{equ:n+1classifier}
%\end{align}
\end{equation}
where $D_k$ is one part of X-DET and $k=1,2,3,4$. Notice that here we remove the LRP detector since it is not differentiable. So that a targeted attacker can generate examples on the classifier and the detectors to perform a white-box attack.
In white-box evaluation, the iteration of PGD is set to 100 and the step size $\alpha$ is set to 0.000781 for the three datasets.
